# Supplementary material for: Computational Prediction of Muon Stopping Sites: a Novel Take on the Unperturbed Electrostatic Potential Method
Source: arXiv:2005.02024 source file (2020-05-05)
Supplement: Supplementary file 1 [file SI.pdf]

# Computational Prediction of Muon Stopping Sites: a Novel Take on the Unperturbed Electrostatic Potential Method - Supplementary Information

Simone Sturniolo, Leandro Liborio

May 5, 2020

In this document we will show an example of how a search for the muon stopping sites could be carried out in  $\text{Fe}_3\text{O}_4$ .

## 1 Run pm-symmetry using $\text{Fe}_3\text{O}_4$ 's structural file.

This would produce an output, with the symmetry analysis of the special Wyckoff positions in  $\text{Fe}_3\text{O}_4$ , that is shown below:

Listing 1: Output of pm-symmetry fe3o4.cell

```
Wyckoff points symmetry report for fe3o4.cell
Space Group International Symbol: Fd-3m
Space Group Hall Number: 525
Absolute                               Fractional                               Hessian constraints
[0. 0. 0.] [0. 0. 0.] none
[0. 2.0895 2.0895] [0. 0.25 0.25] none
[0. 4.179 4.179] [0. 0.5 0.5] none
[0. 6.2685 6.2685] [0. 0.75 0.75] none
[1.04475 1.04475 5.22375] [0.125 0.125 0.625] isotropic
[1.04475 5.22375 1.04475] [0.125 0.625 0.125] isotropic
[2.0895 0. 2.0895] [0.25 0. 0.25] none
[2.0895 2.0895 0. ] [0.25 0.25 0. ] none
[2.0895 4.179 6.2685] [0.25 0.5 0.75] none
[2.0895 6.2685 4.179 ] [0.25 0.75 0.5 ] none
[3.13425 3.13425 3.13425] [0.375 0.375 0.375] isotropic
[3.13425 7.31325 7.31325] [0.375 0.875 0.875] isotropic
[4.179 0. 4.179] [0.5 0. 0.5] none
[4.179 2.0895 6.2685] [0.5 0.25 0.75] none
[4.179 4.179 0. ] [0.5 0.5 0. ] none
[4.179 6.2685 2.0895] [0.5 0.75 0.25] none
```

|    |                           |                     |           |
|----|---------------------------|---------------------|-----------|
| 32 | [5.22375 1.04475 1.04475] | [0.625 0.125 0.125] | isotropic |
| 33 | [5.22375 5.22375 5.22375] | [0.625 0.625 0.625] | isotropic |
| 34 | [6.2685 0. 6.2685]        | [0.75 0. 0.75]      | none      |
| 35 | [6.2685 2.0895 4.179 ]    | [0.75 0.25 0.5 ]    | none      |
| 36 | [6.2685 4.179 2.0895]     | [0.75 0.5 0.25]     | none      |
| 37 | [6.2685 6.2685 0. ]       | [0.75 0.75 0. ]     | none      |
| 38 | [7.31325 3.13425 7.31325] | [0.875 0.375 0.875] | isotropic |
| 39 | [7.31325 7.31325 3.13425] | [0.875 0.875 0.375] | isotropic |

40 As we can see, the list of unoccupied special Wyckoff positions for  $\text{Fe}_3\text{O}_4$  is relatively long. Therefore, the symmetry analysis in this case could be useful only if  
 41 combined with some other piece of known information about the muon stopping site.  
 42 For instance, we may know that the stopping site is placed somewhere along a Wyckoff  
 43 *line* (as it is the case for  $\text{MnSi}$ ). Otherwise, we would need to test each one of these  
 44 positions, which might be impractical because, (as it is the case in  $\text{Fe}_3\text{O}_4$ ), the muon  
 45 stopping site may not be in a Wyckoff position.  
 46

47  
 48 So, for cases like this one, we need to continue the search for potential muon stop-  
 49 ping sites. The next steps in the procedure include: the generation of muonated struc-  
 50 tures with muons in random positions; the relaxation of the muon position in each one  
 51 of this structures and the subsequent performance of a clustering analysis.

## 52 2 Generate Structures with Muons in Random Posi- 53 tions

54 We run `pm-muairss` to generate a set of structure files with muon defects placed in  
 55 random positions. This is done by running the line:

```
56 pm-muairss -t w <fe3o4.cell> <fe3o4.yaml>
```

57 and an example of `fe3o4.yaml` file for running this calculation is:

Listing 2: `fe3o4.yaml`

```
58 poisson_r: 0.6
59 name: fe3o4
60 charged: true
61 geom_steps: 300
62 vdw_scale: 0.25
63 calculator: uep
64 uep_gw_factor: 4.0
65 uep_chden: fe3o4.den_fmt
66 geom_force_tol: 0.05
67 clustering_method: hier
68 clustering_hier_t: 0.2
```

69 The muonated structures generated by this run will be stored in the folders `muon-airss-out/uep/fe3o4_*`,  
70 where `*` is a numerical label that identifies each particular muonated structure. The  
71 number of structures generated by this procedure will depend on the values of param-  
72 eters in the `fe3o4.yaml` file such as `vdw_scale` and `poisson_r`.

73  
74 The next step is to relax each one of these newly generated muonated structures.

### 75 **3 Relaxing the Muon Position in each Structure with** 76 **`pm-uep-opt`**

77 In each one of these newly created `fe3o4_*` folders there will be a new `fe3o4_*.yaml`  
78 file, which will contain instructions for relaxing the muon positions in each one of the  
79 muonated structures by running the library `pm-uep-opt`. Below there is an example  
80 of this `fe3o4_*.yaml` file:

Listing 3: `fe3o4_*.yaml`

```
81 chden_path: path-to-folder
82 chden_seed: fe3o4
83 geom_steps: 300
84 gw_factor: 6.0
85 mu_pos:
86 - 6.6017194506272086
87 - 3.924221192037714
88 - 3.8231862749935717
89 opt_method: trust-exact
90 opt_tol: 0.05
91 particle_mass: 1.67382335232e-27
92 save_pickle: true
```

93 and we relax each one of these structures by running:

```
94 pm-uep-opt <fe3o4_*.yaml>
```

95 for each `fe3o4_*.yaml` in each one of the newly generated folders<sup>1</sup>. The result  
96 will be output in a `fe3o4_*.uep` file such as:

---

<sup>1</sup>If the calculation is being run in Linux, the relaxations could be done, for instance, using a Bash script.

Listing 4: fe3o4\_\*.yaml

```

97
98 *****
99 |  UU  UU  EEEEE  PPPP  |
100 |  UU  UU  EE      PP  PP  |
101 |  UU  UU  EEEEE  PPPP  |
102 |  UU  UU  EE      PP      |
103 |   UUU  EEEEE  PP      |
104 *****
105
106 Unperturbed Electrostatic Potential
107 optimiser for mu+ stopping site finding
108
109 by Simone Sturniolo (2018)
110
111 Calculations started on 2019-12-05 15:24:10.820543
112
113 Charge distribution loaded from ~/Calculations/UEP_Paper/Fe3O4/fe3o4
114 Gaussian width factor used: 6.0
115 Particle mass: 1.67382335232e-27 kg
116
117 -----
118
119 Performing optimisation with method trust-exact
120 Tolerance required for convergence: 0.05 eV
121 Maximum number of steps: 300
122 Defect starting position: 6.6017194506272086 3.924221192037714 3.823186274993571
123
124 -----
125
126 Optimisation stopped after 8 steps
127
128 Final coordinates: 5.789295137667838 4.670038556634775 2.983741171022327 Ang
129 Final fractional coordinates: 0.6926651277420242 0.5587507246512053 0.3569922434
130 Classical energy: -11.47475742543093 eV
131 Zero-point energy: 0.17842078166219383 eV
132 Quantum total energy: -11.296336643768736 eV
133
134 Calculation time: 64.172284 s
135
136 These relaxations may take some time. If the system is small and simple, the re-
137 laxations will be fast. However, if the system is large and sophisticated and there is a
138 large number of structures, these relaxations could be relatively expensive to run.
139
140 In any case, once the relaxations are ready, we need to perform the clustering anal-
141 ysis. This is done by running the line
142
143 pm-muairss -t r <fe3o4.cell> <fe3o4.yaml>

```

141 from the folder where all the structures were generated<sup>2</sup>. This generates two new  
 142 files:

143 • `fe3o4_clusters.text`: This file contains the structures that form each of pre-  
 144 dicted of the clusters that are associated to potential muon stopping sites. This  
 145 file also has information about which would be a representative structural file for  
 146 each stopping site.

147 • `fe3o4_fe3o4_uep_clusters.dat`: This file has the average energy, minimum  
 148 structure energy and standard deviation of the energy for each of the clusters.

149 Examples of this two files are below:

Listing 5: `fe3o4_clusters.text`

```

150
151 *****
152 |                                     |
153 |           MUAIRSS                 |
154 |      Clustering report            |
155 |                                     |
156 *****
157
158 Name: fe3o4
159 Date: 2019-12-05 18:02:33.530251
160 Structure file(s): fe3o4-out.cell
161 Parameter file: fe3o4.yaml
162
163 Clustering method: Hierarchical
164     t = 0.2
165
166
167 *****
168
169 Clusters for fe3o4:
170 CALCULATOR: uep
171     2 clusters found
172
173
174     _____
175     Cluster 1
176     _____
177     Structures: 13
178
179     Energy (eV):
180     Minimum      Average      StDev
  
```

<sup>2</sup>In our case, this is the folder from where we can see the `muon-airss-out` folder.

```

181      -9.90          -9.90          0.00
182
183      Minimum energy structure : fe3o4_29
184
185
186      Structure list :
187      fe3o4_2 fe3o4_13          fe3o4_14          fe3o4_29
188      fe3o4_38          fe3o4_57          fe3o4_73          fe3o4_88
189      fe3o4_115          fe3o4_120          fe3o4_132          fe3o4_137
190      fe3o4_145
191
192      _____
193      Cluster 2
194      _____
195      Structures : 139
196
197      Energy (eV):
198      Minimum          Average          StDev
199      -11.47          -11.47          0.00
200
201      Minimum energy structure : fe3o4_48
202
203
204      Structure list :
205      fe3o4_1 fe3o4_3 fe3o4_4 fe3o4_5
206      fe3o4_6 fe3o4_7 fe3o4_8 fe3o4_9
207      fe3o4_10          fe3o4_11          fe3o4_12          fe3o4_15
208      fe3o4_16          fe3o4_17          fe3o4_18          fe3o4_19
209      fe3o4_20          fe3o4_21          fe3o4_22          fe3o4_23
210      fe3o4_24          fe3o4_25          fe3o4_26          fe3o4_27
211      fe3o4_28          fe3o4_30          fe3o4_31          fe3o4_32
212      fe3o4_33          fe3o4_34          fe3o4_35          fe3o4_36
213      fe3o4_37          fe3o4_39          fe3o4_40          fe3o4_41
214      fe3o4_42          fe3o4_43          fe3o4_44          fe3o4_45
215      fe3o4_46          fe3o4_47          fe3o4_48          fe3o4_49
216      fe3o4_50          fe3o4_51          fe3o4_52          fe3o4_53
217      fe3o4_54          fe3o4_55          fe3o4_56          fe3o4_58
218      fe3o4_59          fe3o4_60          fe3o4_61          fe3o4_62
219      fe3o4_63          fe3o4_64          fe3o4_65          fe3o4_66
220      fe3o4_67          fe3o4_68          fe3o4_69          fe3o4_70
221      fe3o4_71          fe3o4_72          fe3o4_74          fe3o4_75
222      fe3o4_76          fe3o4_77          fe3o4_78          fe3o4_79
223      fe3o4_80          fe3o4_81          fe3o4_82          fe3o4_83
224      fe3o4_84          fe3o4_85          fe3o4_86          fe3o4_87
225      fe3o4_89          fe3o4_90          fe3o4_91          fe3o4_92
226      fe3o4_93          fe3o4_94          fe3o4_95          fe3o4_96

```

```

227      fe3o4_97      fe3o4_98      fe3o4_99      fe3o4_100
228      fe3o4_101     fe3o4_102     fe3o4_103     fe3o4_104
229      fe3o4_105     fe3o4_106     fe3o4_107     fe3o4_108
230      fe3o4_109     fe3o4_110     fe3o4_111     fe3o4_112
231      fe3o4_113     fe3o4_114     fe3o4_116     fe3o4_117
232      fe3o4_118     fe3o4_119     fe3o4_121     fe3o4_122
233      fe3o4_123     fe3o4_124     fe3o4_125     fe3o4_126
234      fe3o4_127     fe3o4_128     fe3o4_129     fe3o4_130
235      fe3o4_131     fe3o4_133     fe3o4_134     fe3o4_135
236      fe3o4_136     fe3o4_138     fe3o4_139     fe3o4_140
237      fe3o4_141     fe3o4_142     fe3o4_143     fe3o4_144
238      fe3o4_146     fe3o4_147     fe3o4_148     fe3o4_149
239      fe3o4_150     fe3o4_151     fe3o4_152

```

240

241

242

243 Similarity (ranked):

244 0 <--> 1 (distance = 1.602)

245

246

247

248

249 =====

Listing 6: fe3o4\_fe3o4\_uep\_clusters.dat

```

250      1      13      -9.897753370173747      -9.897721148028158
251      5.260352456001172e-05
252      2      139      -11.474801196064512      -11.474700683287459
253      0.00015287319327130454

```
